# Supplementary material for: ASASSN-16eg: New candidate of long-period WZ Sge-type dwarf nova
Source: arXiv:1708.09206 ancillary file (2017-09-22)
Supplement: Supplementary file 1 [file a16egsi.pdf]

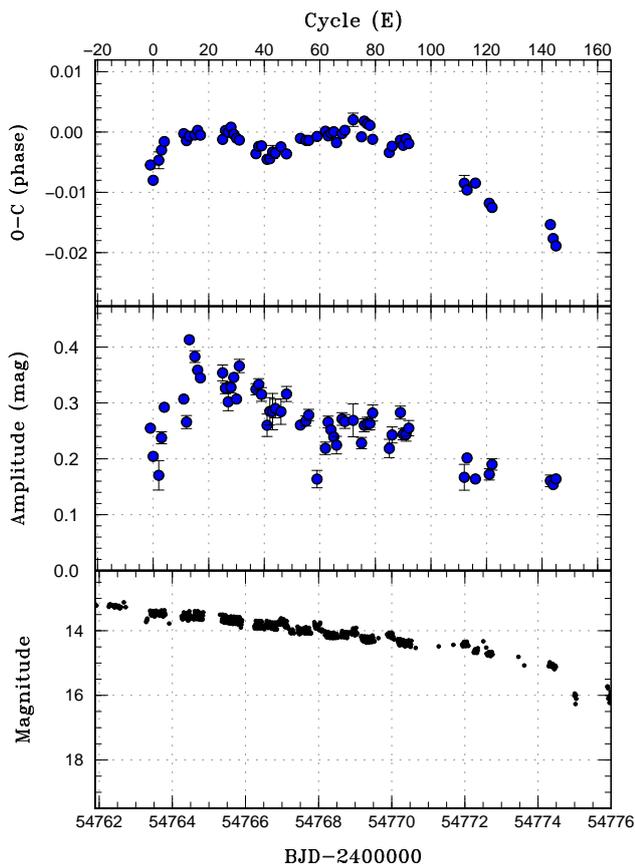

**Fig. S1.** Upper panel: The  $O - C$  curve of V1251 Cyg during BJD 2454763–2454776. We used an ephemeris of BJD  $2454765.6790 + 0.0759607E$  for drawing this figure. Middle panel: The amplitude of superhumps. Lower panel: The light curve. The horizontal axis in units of BJD and cycle number is common to all of these panels.

## Supplementary Discussion

V1251 Cyg has shown 5 superoutbursts in 1963, 1991, 1994, 1997 and 2008 (Weber 1966; Wenzel 1991; Kato 1995; Kato et al. 2009). The supercycle seems to be 3–28 yr. Rebrightenings were observed in the 1997 and 2008 superoutbursts and in the 2008 superoutburst, double-wave variations similar to early superhumps were observed (Kato et al. 2009). Kato et al. (2009) analyzed the 2008 superoutburst of V1251 Cyg and found the period of early superhumps to be 0.07433(6).

We reanalyzed the 2008 superoutburst of V1251 Cyg by using VSNET and AAVSO data. The times of maxima of ordinary superhumps are listed in table S3. Figure S1 shows the  $O - C$  curve, the amplitude of superhumps (middle panel) and the light curve (lower panel) of V1251 Cyg during BJD 2454763–2454776. We regarded BJD 2454763.2–2454764.9 ( $0 \leq E \leq 17$ ) as stage A from the variation of the superhump period and the amplitude of superhumps. Figure S2 shows the result of PDM analysis of stage A superhumps (upper panel) and

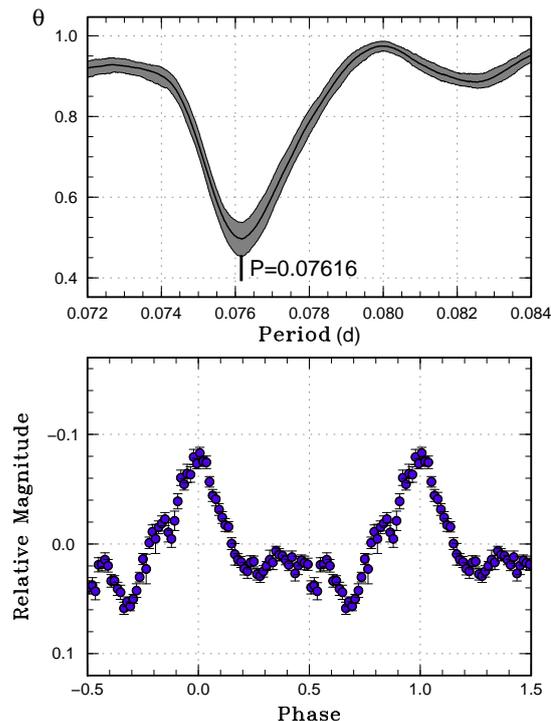

**Fig. S2.** Upper panel:  $\theta$ -diagram of our PDM analysis of stage A superhumps of V1251 Cyg (BJD 2454763.2–2454764.9). Lower panel: Phase-averaged profile of stage A superhumps.

the mean profile (lower panel). We found the stage A superhump period to be 0.07616(3) d. We also attempt to estimate the period of early superhumps but failed because of a shortage of observational data and contamination by inaccurate data. Although double-wave variations of magnitude similar to early superhumps can be seen in its light curve before the appearance of ordinary superhumps, it is so contaminated that we could not obtain a reliable period of early superhumps.

RZ Leo has shown many superoutbursts. The brightenings of RZ Leo are recorded in 1918, 1935, 1952, 1976, 1984, 1987, 1988, 1989, 1990, 2000, 2006 and 2016 (Wolf 1919; Richter 1985; Ishioka et al. 2001; Kato 2015; Kato et al. 2016). In these recorded brightenings, the 1989 brightening seems to be a normal outburst (Narumi et al. 1989; O’Donoghue et al. 1991). In addition, Ishioka et al. (2001) indicated that the 1987, 1988, 1989 and 1990 brightenings might be short and probably were mistaken as brightenings of another nearby object. Therefore, the superoutbursts seem to be in 1918, 1935, 1952, 1976, 1984, 2000, 2006 and 2016, and thus the supercycle seems to be 6–24 yr. Although RZ Leo had shown many superoutbursts, variations of magnitude similar to early superhumps are recorded only in the 2000 superoutbursts (Ishioka et al. 2001; Kato et al. 2016). The spectroscopic orbital period is 0.07651(26) d (Mennickent, Tappert 2001) and the photometric period is 0.0756(12) d (Mennickent et al. 1999). Ishioka

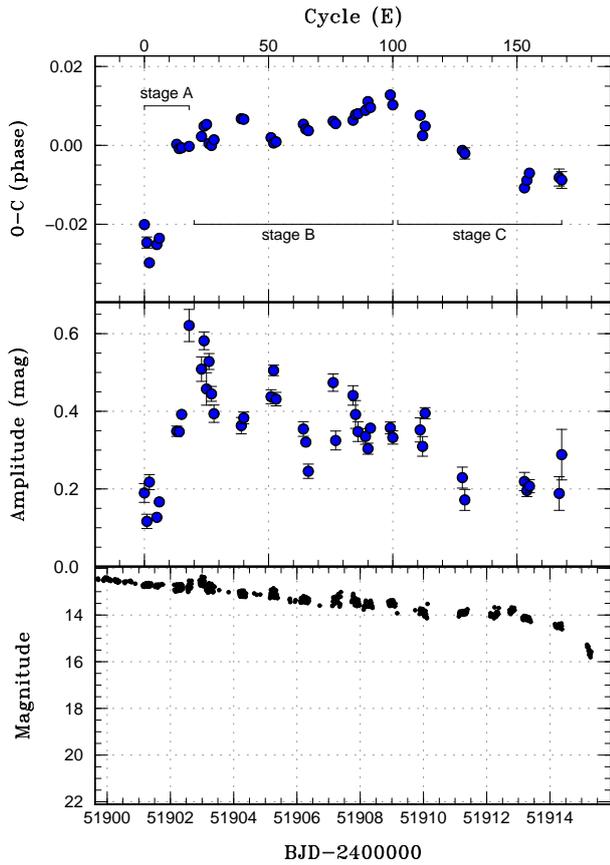

**Fig. S3.** Upper panel: The  $O - C$  curve of RZ Leo during BJD 2451901–2451915. We used an ephemeris of BJD 2451902.2763+0.0785326 $E$  for drawing this figure. Middle panel: The amplitude of superhumps. Lower panel: The light curve. The horizontal axis in units of BJD and cycle number is common to all of these panels.

et al. (2001) analyzed the 2000 superoutburst of RZ Leo and found the orbital period to be 0.07616(21) d, and estimated the mass ratio to be 0.14 from the period of early superhumps and the superhump excess.

We reanalyzed the 2000 superoutburst of RZ Leo by using VSNET and AAVSO data and estimated the mass ratio by using a new method developed by Kato, Osaki (2013). The times of maxima of ordinary superhumps are listed in table S4. Figure S3 shows the  $O - C$  curve, the amplitude of superhumps (middle panel) and the light curve (lower panel) of RZ Leo during BJD 2451901–2451915. We regarded BJD 2451901.1–2451902.7 ( $0 \leq E \leq 18$ ) as stage A from the variation of the superhump period and the amplitude of superhumps. Figures S4 and S5 show the results of PDM analysis of early superhumps and stage A superhumps (upper panel) and the mean profiles (lower panel), respectively. We found the period of early superhumps to be 0.07626(7) d and the stage A superhump period to be 0.08072(5) d, and then we estimate the mass ratio at 0.165(6)

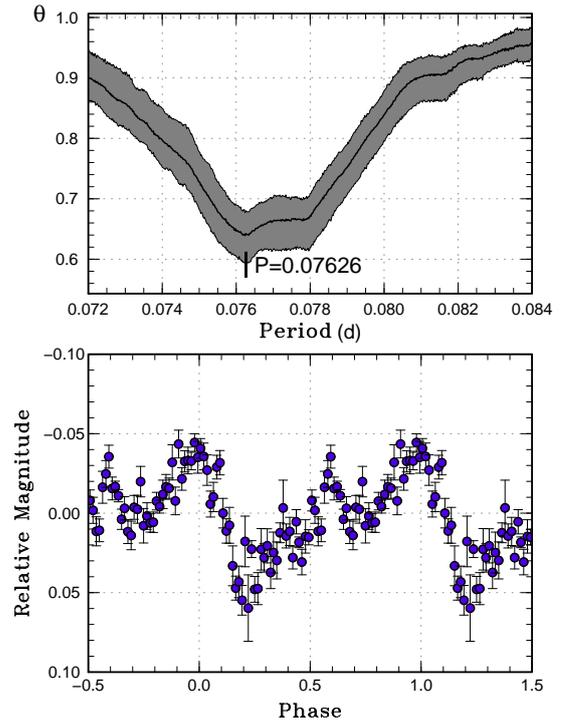

**Fig. S4.** Upper panel:  $\theta$ -diagram of our PDM analysis of early superhumps of RZ Leo (BJD 2451899.1–2451901.0). Lower panel: Phase-averaged profile of early superhumps.

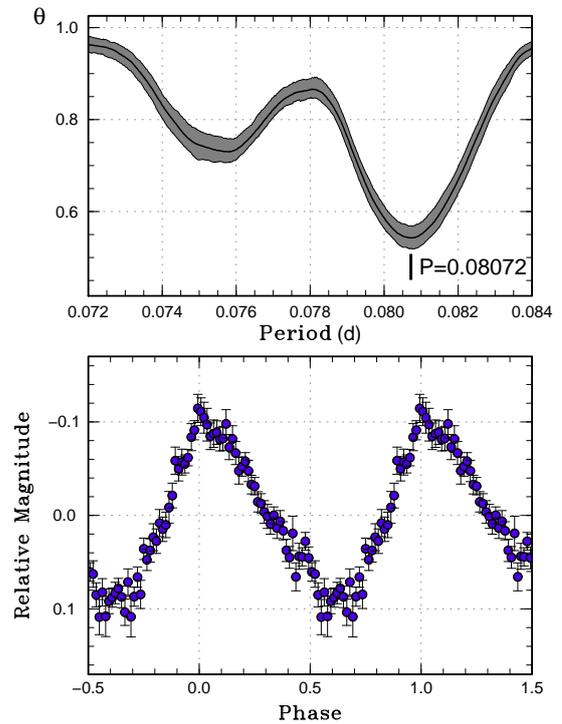

**Fig. S5.** Upper panel:  $\theta$ -diagram of our PDM analysis of stage A superhumps of RZ Leo (BJD 2451901.1–2451902.7). Lower panel: Phase-averaged profile of stage A superhumps.

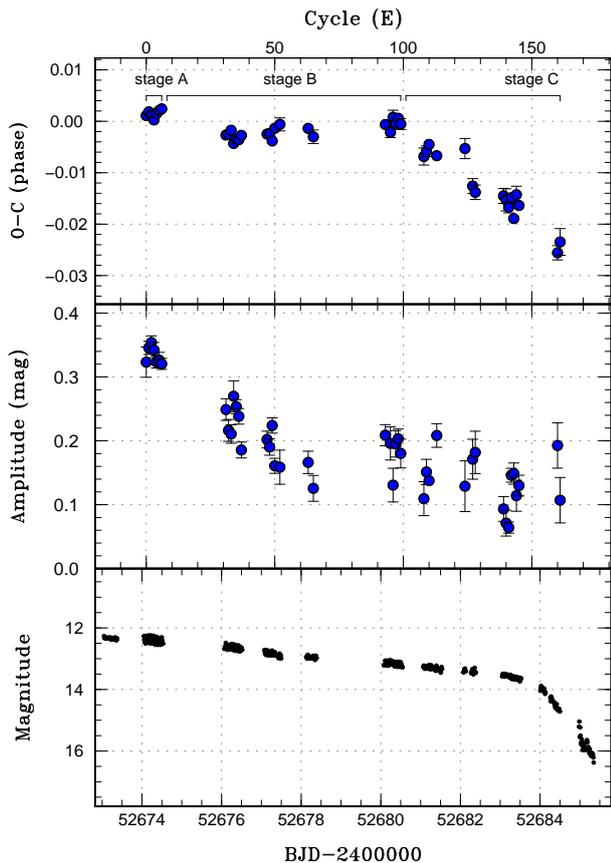

**Fig. S6.** Upper panel: The  $O - C$  curve of BC UMa during BJD 2452674–2452685. We used an ephemeris of BJD 2452674.2372+0.0645728 $E$  for drawing this figure. Middle panel: The amplitude of superhumps. Lower panel: The light curve. The horizontal axis in units of BJD and cycle number is common to all of these panels.

by using these periods. The period of early superhumps is consistent with that obtained by Ishioka et al. (2001) within the errors. The mass ratio we obtained is slightly larger than  $q = 0.14$  that Ishioka et al. (2001) calculated from the superhump excess. It should be noted that this estimated mass ratio involves slightly larger uncertainties because of the short baseline of the data of stage A superhumps.

BC UMa has shown many superoutbursts and early superhumps were observed. The superoutbursts of BC UMa were recorded in 1960, 1962, 1982, 1990, 1992, 1994, 2000, 2003 and 2009 (Romano 1964; Kunjaya et al. 1998; Boyd 2003; Maehara et al. 2007; Kato et al. 2009; Kato et al. 2010; Kato 2015). The supercycle of BC UMa is thus about 2–20 yr. Patterson et al. (2003) found the orbital period to be 0.062605(11) d and the period of early superhumps to be 0.06256(8) d from the 2000 superoutburst. Maehara et al. (2007) analyzed the 2003 superoutburst and found the period of early superhumps to be 0.06258(13) d, and estimated the mass

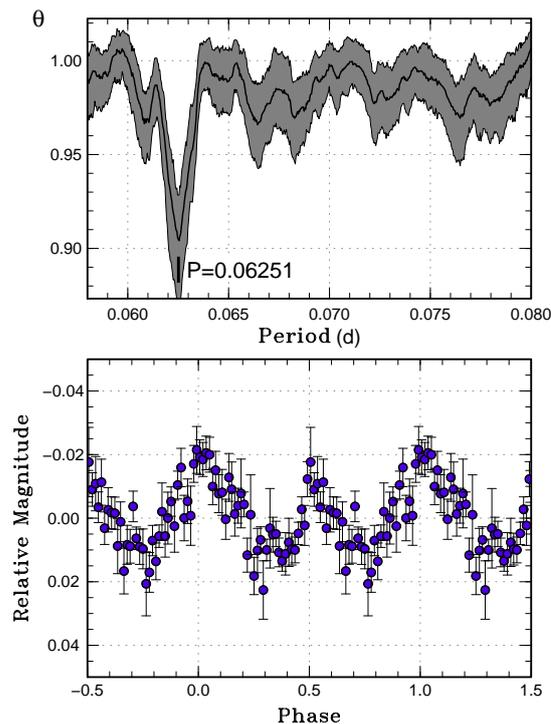

**Fig. S7.** Upper panel:  $\theta$ -diagram of our PDM analysis of early superhumps of BC UMa (BJD 2452672.1–2452673.4). Lower panel: Phase-averaged profile of early superhumps.

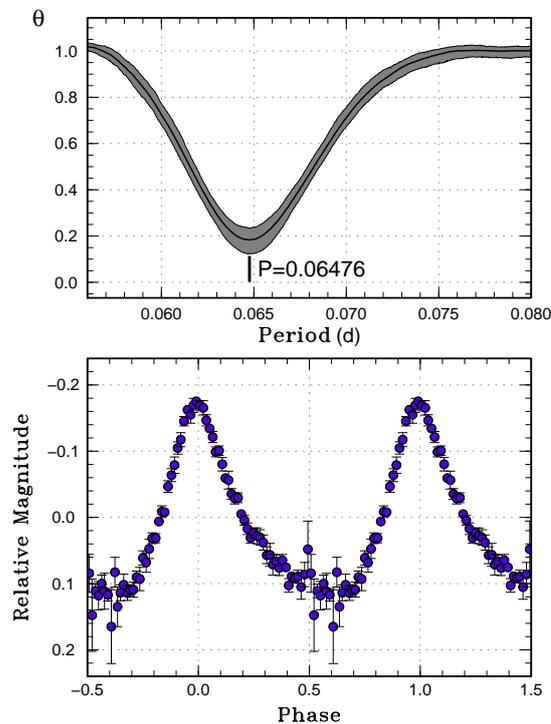

**Fig. S8.** Upper panel:  $\theta$ -diagram of our PDM analysis of stage A superhumps of BC UMa (BJD 2452674.0–2452674.6). Lower panel: Phase-averaged profile of stage A superhumps.

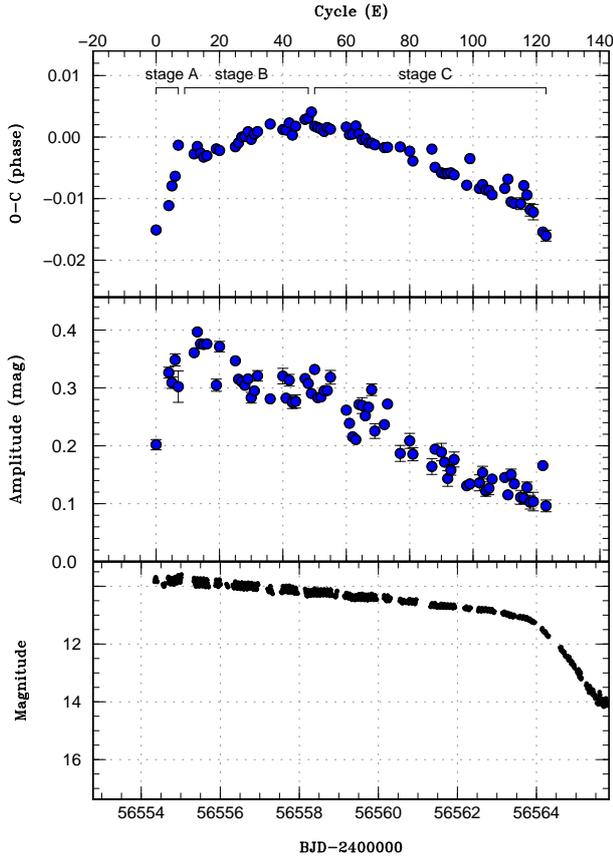

**Fig. S9.** Upper panel: The  $O - C$  curve of MASTER J004527 during BJD 2456554–2456565. We used an ephemeris of BJD  $2456556.3815 + 0.0801953E$  for drawing this figure. Middle panel: The amplitude of superhumps. Lower panel: The light curve. The horizontal axis in units of BJD and cycle number is common to all of these panels.

ratio to be  $q = 0.13$  from the superhump excess. They also suggested that BC UMa may be an intermediate class between the WZ Sge type DNe and the SU UMa-type ones from the presence of normal outbursts and two types of superoutbursts. One has long duration and large amplitude comparable to WZ Sge-type DNe and the other has short duration and small amplitude in comparison with WZ Sge-type ones, which are supposed to reflect the stored mass in the disk before each superoutburst.

We reanalyzed the 2003 superoutburst of BC UMa for the purpose of the estimation of its mass ratio by using the new method proposed in Kato, Osaki (2013). The times of maxima of ordinary superhumps are listed in table S5. Figure S6 shows the  $O - C$  curve, the amplitude of superhumps (middle panel) and the light curve (lower panel) of BC UMa during BJD 2452674–2452685. We regarded BJD 2452674.0–2452674.6 ( $0 \leq E \leq 6$ ) as stage A from the variation of the superhump period and the amplitude of superhumps. Figures S7 and S8 show the results of PDM analysis of early superhumps and stage A super-

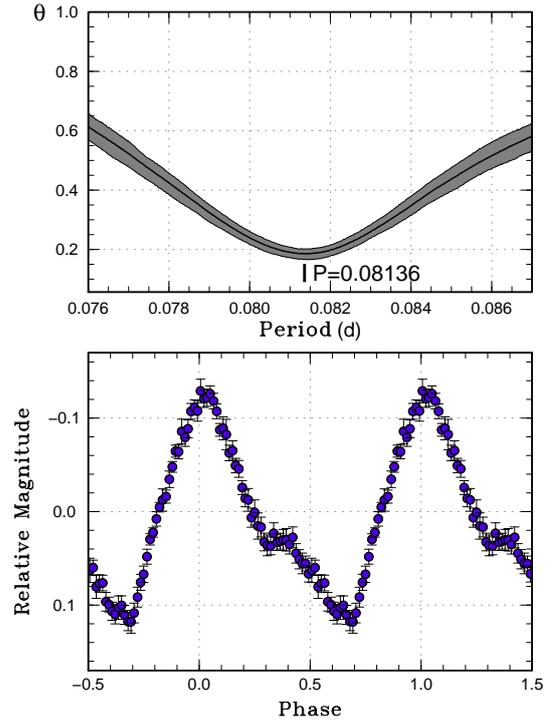

**Fig. S10.** Upper panel:  $\theta$ -diagram of our PDM analysis of stage A superhumps of MASTER J004527 (BJD 2456554.3–56555.1). Lower panel: Phase-averaged profile of stage A superhumps.

humps (upper panel) and the superhump profiles (lower panel), respectively. We found the period of early superhumps to be  $0.06251(5)$  d, and naturally, this value is consistent with the period in Maehara et al. (2007) within the errors. We obtained the stage A superhump period to be  $0.06476(7)$  d. We then estimated the mass ratio to be  $0.096(6)$ , which is smaller than that in Maehara et al. (2007) and larger than the upper limit of mass ratios for occurrence of the 2:1 resonance.

MASTER OT J004527.52+503213.8 (hereafter MASTER J004527) is regarded as WZ Sge-type DNe based on the large outburst amplitude, and only one superoutburst in 2013 is recorded (Kato et al. 2014). Amplitudes of superhumps is much larger than those of period bouncers and thus this object may not be a period bouncer.

We reanalyzed the 2013 superoutburst of MASTER J004527. The times of maxima of ordinary superhumps are listed in table S6. Figure S9 shows the  $O - C$  curve, the amplitude of superhumps (middle panel) and the light curve (lower panel) of MASTER J004527 during BJD 2456554–2456565. We regarded BJD 2456554.3–2456555.1 ( $0 \leq E \leq 7$ ) as stage A from the variation of the superhump period and the amplitude of superhumps. Figure S10 shows the result of PDM analysis of stage A superhumps (upper panel) and the superhump profile (lower panel). We found the stage A superhump period to be  $0.08136(7)$  d.

QY Per is regarded as a WZ Sge-type DN from the large outburst amplitude and long recurrence time (Kato et al. 2009; Kato et al. 2016). This object showed three superoutbursts in 1999, 2005 and 2015 and thus the supercycle is 6–10 years. The 2015 superoutburst seems to have shown no early superhumps. It appears that this object showed a different type of superoutburst (Kato et al. 2016).

We attempted to obtain the stage A superhump period from the 1999 superoutburst but failed because of the shortage of observational data.

## References

- Boyd, D. 2003, *J. Br. Astron. Assoc.*, 113, 208  
 Ishioka, R., et al. 2001, *PASJ*, 53, 905  
 Kato, T. 1995, *IBVS*, 4152  
 Kato, T. 2015, *PASJ*, 67, 108  
 Kato, T., et al. 2014, *PASJ*, 66, 90  
 Kato, T., et al. 2016, *PASJ*, in press (arXiv/1605.06221)  
 Kato, T., et al. 2009, *PASJ*, 61, S395  
 Kato, T., et al. 2010, *PASJ*, 62, 1525  
 Kato, T., & Osaki, Y. 2013, *PASJ*, 65, 115  
 Kunjaya, C., Kato, T., & Hirata, R. 1998, *Highlights of Astronomy*, 11, 388  
 Maehara, H., Hachisu, I., & Nakajima, K. 2007, *PASJ*, 59, 227  
 Mennickent, R. E., Sterken, C., Gieren, W., & Unda, E. 1999, *A&A*, 352, 239  
 Mennickent, R. E., & Tappert, C. 2001, *A&A*, 372, 563  
 Narumi, H., Korth, S., Dyck, G., Iida, M., & Hurst, G. 1989, *IAU Circ.*, 4757  
 O'Donoghue, D., Chen, A., Marang, F., Mittaz, J. P. D., Winkler, H., & Warner, B. 1991, *MNRAS*, 250, 363  
 Patterson, J., et al. 2003, *PASP*, 115, 1308  
 Richter, G. A. 1985, *IBVS*, 2714  
 Romano, G. 1964, *Mem. Soc. Astron. Ital.*, 35, 101  
 Weber, R. 1966, *IBVS*, 123  
 Wenzel, W. 1991, *IBVS*, 3689  
 Wolf, M. 1919, *Astron. Nachr.*, 209, 85

**Table S1.** Log of observations of ASASSN-16eg.

| Start*  | End*    | mag <sup>†</sup> | error <sup>‡</sup> | $N^{\S}$ | obs <sup>  </sup> | sys <sup>#</sup> |
|---------|---------|------------------|--------------------|----------|-------------------|------------------|
| 89.4093 | 89.5309 | -0.320           | 0.002              | 204      | Van               | C                |
| 90.2630 | 90.3258 | -0.762           | 0.003              | 156      | KU1               | C                |
| 90.3915 | 90.3955 | 13.009           | 0.005              | 6        | BPO               | CV               |
| 90.4401 | 90.4906 | 12.859           | 0.003              | 132      | Trt               | CV               |
| 90.4854 | 90.6306 | -0.153           | 0.001              | 330      | Van               | C                |
| 90.6317 | 90.8780 | 12.853           | 0.002              | 253      | UJH               | CV               |
| 90.6897 | 90.9264 | 13.157           | 0.001              | 458      | BJA               | CV               |
| 91.3734 | 91.5569 | 13.240           | 0.002              | 243      | Han               | CV               |
| 91.4236 | 91.4825 | 13.018           | 0.002              | 157      | Trt               | CV               |
| 91.6305 | 91.8529 | 13.028           | 0.005              | 133      | UJH               | CV               |
| 92.3479 | 92.6688 | 13.448           | 0.001              | 383      | BPO               | CV               |
| 92.3834 | 92.5556 | 13.452           | 0.001              | 253      | Han               | CV               |
| 92.4047 | 92.5911 | 0.276            | 0.001              | 424      | Van               | C                |
| 92.6635 | 92.8786 | 13.232           | 0.002              | 242      | UJH               | CV               |
| 92.6854 | 92.8961 | 13.315           | 0.001              | 250      | CMJ               | V                |
| 92.6897 | 92.9280 | 13.531           | 0.001              | 443      | BJA               | CV               |
| 92.8935 | 92.9646 | 13.203           | 0.011              | 42       | SGE               | CV               |
| 93.0910 | 93.3325 | 0.384            | 0.002              | 340      | Aka               | C                |
| 93.3844 | 93.5587 | 13.599           | 0.001              | 270      | Han               | CV               |
| 93.4689 | 93.6118 | 13.355           | 0.001              | 386      | Trt               | CV               |
| 93.5587 | 93.9208 | 13.873           | 0.002              | 398      | SDB               | CV               |
| 93.6313 | 93.8754 | 13.368           | 0.002              | 267      | UJH               | CV               |
| 93.6644 | 93.9031 | 13.446           | 0.001              | 353      | CMJ               | V                |
| 93.7261 | 93.8841 | 13.799           | 0.001              | 295      | MZK               | CV               |
| 93.7271 | 93.7868 | 13.428           | 0.015              | 10       | Neu               | V                |
| 93.8262 | 93.9963 | 13.343           | 0.003              | 152      | SGE               | CV               |
| 94.1120 | 94.2159 | 0.519            | 0.004              | 74       | Aka               | C                |
| 94.2207 | 94.3124 | 13.651           | 0.003              | 195      | Ioh               | C                |
| 94.4401 | 94.6122 | 13.425           | 0.002              | 468      | Trt               | CV               |
| 94.6297 | 94.8736 | 13.445           | 0.003              | 268      | UJH               | CV               |
| 94.6366 | 94.9024 | 13.527           | 0.003              | 382      | CMJ               | V                |
| 94.7388 | 95.0308 | 13.730           | 0.003              | 568      | JJI               | CV               |
| 94.7470 | 94.8895 | 13.883           | 0.004              | 270      | MZK               | CV               |
| 94.7613 | 94.9640 | 13.523           | 0.012              | 32       | Neu               | V                |
| 94.8866 | 95.0007 | 13.429           | 0.005              | 175      | SGE               | CV               |
| 95.0935 | 95.1498 | 13.728           | 0.009              | 124      | Kis               | C                |
| 95.2966 | 95.4441 | 0.115            | 0.007              | 200      | CRI               | C                |
| 95.3693 | 95.5969 | 0.584            | 0.006              | 290      | DPV               | C                |
| 95.3862 | 95.4936 | 13.834           | 0.010              | 64       | Han               | CV               |
| 95.4556 | 95.6518 | 13.598           | 0.005              | 359      | IMi               | CV               |
| 95.5360 | 95.6827 | 13.604           | 0.007              | 202      | RPc               | V                |
| 95.5558 | 95.8947 | 14.061           | 0.005              | 400      | SDB               | CV               |
| 95.5780 | 95.9027 | 13.621           | 0.005              | 480      | CMJ               | V                |
| 95.6314 | 95.8746 | 13.544           | 0.006              | 269      | UJH               | CV               |

\*BJD–2457400.

<sup>†</sup>Mean magnitude.

<sup>‡</sup> $1\sigma$  of the mean magnitude.

<sup>§</sup>Number of observations.

<sup>||</sup>Observer's code: Neu (V. Neustroev team), Van (T. Vanmunster), KU1 (Kyoto U., campus obs.), Trt (T. Tordai), Han (Hankasalmi Obs., by A. Oksanen), Aka (H. Akazawa, OUS), Ioh (H. Itoh), Kis (S. Kiyota), CRI (Crimean Astrophys. Obs.), DPV (P. Dubovsky), IMi (I. Miller), RPc (R. Pickard) and AAVSO collaboration.

<sup>#</sup>Filter. "C" means no filter (clear).

**Table S1.** Log of observations of ASASSN-16eg (continued).

| Start*  | End*    | mag <sup>†</sup> | error <sup>‡</sup> | N <sup>§</sup> | obs <sup>  </sup> | sys <sup>#</sup> |
|---------|---------|------------------|--------------------|----------------|-------------------|------------------|
| 95.6683 | 95.8868 | 13.465           | 0.005              | 439            | RIT               | CV               |
| 95.7350 | 95.9283 | 13.593           | 0.018              | 32             | Neu               | V                |
| 95.7366 | 96.0347 | 13.796           | 0.005              | 384            | JJI               | CV               |
| 95.7462 | 95.8886 | 13.992           | 0.006              | 270            | MZK               | CV               |
| 95.8664 | 96.0175 | 13.484           | 0.007              | 225            | SGE               | CV               |
| 95.9414 | 95.9742 | 13.635           | 0.023              | 30             | FJQ               | V                |
| 95.9439 | 95.9766 | 13.451           | 0.023              | 30             | FJQ               | B                |
| 95.9464 | 95.9791 | 13.606           | 0.024              | 30             | FJQ               | I                |
| 96.0548 | 96.1916 | 0.056            | 0.007              | 235            | KU1               | C                |
| 96.0578 | 96.2629 | 13.787           | 0.008              | 404            | Kis               | C                |
| 96.1035 | 96.3189 | 0.598            | 0.008              | 183            | Aka               | C                |
| 96.1277 | 96.2813 | 13.746           | 0.007              | 274            | Ioh               | C                |
| 96.2862 | 96.4033 | 0.156            | 0.007              | 159            | CRI               | C                |
| 96.3865 | 96.6420 | 0.632            | 0.005              | 403            | Van               | C                |
| 96.4372 | 96.5458 | 13.579           | 0.006              | 257            | Trt               | CV               |
| 96.4803 | 96.6364 | 13.616           | 0.005              | 300            | IMi               | CV               |
| 96.5763 | 96.9059 | 13.663           | 0.005              | 456            | CMJ               | V                |
| 96.5828 | 96.9283 | 14.104           | 0.005              | 415            | SDB               | CV               |
| 96.6250 | 96.8747 | 13.580           | 0.006              | 276            | UJH               | CV               |
| 96.6661 | 96.8412 | 13.701           | 0.006              | 291            | DKS               | CV               |
| 96.7195 | 96.9013 | 13.513           | 0.005              | 394            | RIT               | CV               |
| 96.7291 | 97.0213 | 13.857           | 0.004              | 551            | JJI               | CV               |
| 96.7344 | 96.7916 | 13.604           | 0.032              | 10             | Neu               | V                |
| 96.7624 | 97.0165 | 13.564           | 0.005              | 375            | SGE               | CV               |
| 96.7732 | 96.9646 | 13.705           | 0.007              | 230            | GFB               | V                |
| 96.8806 | 96.9795 | 13.720           | 0.011              | 71             | FJQ               | V                |
| 96.8831 | 96.9820 | 13.604           | 0.012              | 75             | FJQ               | B                |
| 96.8856 | 96.9770 | 13.696           | 0.011              | 72             | FJQ               | I                |
| 97.2118 | 97.3228 | 0.756            | 0.009              | 78             | Aka               | C                |
| 97.3548 | 97.6611 | 14.019           | 0.004              | 372            | BPO               | CV               |
| 97.3786 | 97.4280 | 0.802            | 0.009              | 82             | Van               | C                |
| 97.7311 | 98.0273 | 14.050           | 0.003              | 575            | JJI               | CV               |
| 97.7597 | 98.0115 | 13.748           | 0.004              | 375            | SGE               | CV               |
| 97.8657 | 97.9663 | 13.908           | 0.014              | 39             | FJQ               | V                |
| 97.8682 | 97.9689 | 13.809           | 0.017              | 39             | FJQ               | B                |
| 97.8735 | 97.9638 | 13.878           | 0.015              | 36             | FJQ               | I                |
| 98.1123 | 98.3056 | 14.106           | 0.004              | 413            | Ioh               | C                |
| 98.1250 | 98.3075 | 0.363            | 0.004              | 508            | KU1               | C                |
| 98.3869 | 98.6416 | 0.940            | 0.004              | 404            | Van               | C                |
| 98.4471 | 98.6381 | 13.917           | 0.004              | 370            | IMi               | CV               |
| 98.5048 | 98.6048 | 13.913           | 0.004              | 270            | Trt               | CV               |
| 98.5857 | 98.7635 | 13.994           | 0.005              | 239            | CMJ               | V                |
| 98.6752 | 98.8918 | 13.814           | 0.003              | 471            | RIT               | CV               |
| 98.7009 | 98.8318 | 13.972           | 0.016              | 22             | Neu               | V                |

\*BJD–2457400.

†Mean magnitude.

‡1 $\sigma$  of the mean magnitude.

§Number of observations.

||Observer's code: RIT (M. Richmond), Neu (V. Neustroev team), KU1 (Kyoto U., campus obs.), Kis (S. Kiyota), Aka (H. Akazawa, OUS), Ioh (H. Itoh), CRI (Crimean Astrophys. Obs.), Van (T. Vanmunster), Trt (T. Tordai) IMi (I. Miller) and AAVSO collaboration.

#Filter. "C" means no filter (clear).

**Table S1.** Log of observations of ASASSN-16eg (continued).

| Start*   | End*     | mag <sup>†</sup> | error <sup>‡</sup> | N <sup>§</sup> | obs <sup>  </sup> | sys <sup>#</sup> |
|----------|----------|------------------|--------------------|----------------|-------------------|------------------|
| 98.7310  | 98.7638  | 14.242           | 0.006              | 65             | JJI               | CV               |
| 98.7569  | 99.0205  | 13.845           | 0.004              | 400            | SGE               | CV               |
| 99.4120  | 99.6418  | 1.014            | 0.004              | 363            | Van               | C                |
| 100.3629 | 100.4249 | 14.388           | 0.008              | 57             | Han               | CV               |
| 100.5045 | 100.5554 | 14.225           | 0.005              | 71             | Trt               | CV               |
| 100.7198 | 100.9118 | 14.189           | 0.015              | 32             | Neu               | V                |
| 101.0525 | 101.3187 | 0.663            | 0.003              | 711            | KU1               | C                |
| 102.3653 | 102.4669 | 14.565           | 0.008              | 89             | Han               | CV               |
| 102.6945 | 102.8869 | 14.444           | 0.012              | 32             | Neu               | V                |
| 103.4847 | 103.6973 | 14.688           | 0.004              | 258            | deM               | C                |
| 103.7050 | 103.8968 | 14.497           | 0.013              | 32             | Neu               | V                |
| 104.1938 | 104.3125 | 0.936            | 0.004              | 329            | KU1               | C                |
| 104.5506 | 104.6985 | 14.775           | 0.005              | 169            | deM               | C                |
| 104.7136 | 104.7944 | 14.595           | 0.016              | 14             | Neu               | V                |
| 105.6888 | 105.8832 | 14.748           | 0.009              | 32             | Neu               | V                |
| 106.5020 | 106.6276 | 1.821            | 0.003              | 153            | Van               | C                |
| 107.8014 | 107.9083 | 15.069           | 0.010              | 18             | Neu               | V                |
| 108.1021 | 108.3142 | 2.293            | 0.008              | 102            | Aka               | C                |
| 108.2283 | 108.3125 | 1.787            | 0.003              | 366            | KU1               | C                |
| 108.7084 | 108.9025 | 15.971           | 0.022              | 32             | Neu               | V                |
| 109.1621 | 109.3116 | 3.597            | 0.016              | 72             | Aka               | C                |
| 109.1985 | 109.2805 | 2.908            | 0.005              | 229            | KU1               | C                |
| 110.1797 | 110.1929 | 3.622            | 0.033              | 32             | KU1               | C                |
| 111.6673 | 111.6673 | 17.791           | 0.05               | 6              | Neu               | V                |
| 112.4593 | 112.6131 | 4.024            | 0.012              | 128            | Van               | C                |
| 112.7011 | 112.8398 | 16.264           | 0.072              | 15             | Neu               | V                |
| 113.1365 | 113.1419 | 1.901            | 0.008              | 13             | KU1               | C                |
| 113.3565 | 113.6137 | 2.634            | 0.003              | 318            | Van               | C                |
| 113.6668 | 113.8069 | 15.934           | 0.019              | 15             | Neu               | V                |
| 114.6896 | 114.6896 | 17.466           | 0.04               | 6              | Neu               | V                |
| 115.8809 | 115.8809 | 18.401           | 0.04               | 6              | Neu               | V                |
| 119.8117 | 119.8117 | 18.710           | 0.18               | 6              | Neu               | V                |
| 120.1786 | 120.1939 | 18.500           | 0.000              | 2              | KU1               | C                |
| 122.7220 | 122.7220 | 18.840           | 0.15               | 6              | Neu               | V                |
| 152.8352 | 152.8352 | 19.100           | 0.04               | 6              | Neu               | V                |
| 154.7665 | 154.7665 | 19.162           | 0.04               | 6              | Neu               | V                |
| 155.6973 | 155.6973 | 19.194           | 0.04               | 6              | Neu               | V                |
| 157.6497 | 157.6497 | 19.198           | 0.04               | 6              | Neu               | V                |
| 160.6502 | 160.6502 | 19.220           | 0.04               | 6              | Neu               | V                |
| 204.6500 | 204.6500 | 19.470           | 0.04               | 6              | Neu               | V                |
| 236.6107 | 236.6107 | 19.472           | 0.04               | 6              | Neu               | V                |
| 242.6929 | 242.6929 | 19.484           | 0.01               | 6              | Neu               | V                |
| 267.5930 | 267.5930 | 19.635           | 0.08               | 6              | Neu               | V                |
| 301.3372 | 301.3372 | 19.560           | 0.01               | 6              | Neu               | V                |

\*BJD–2457400.

†Mean magnitude.

‡1 $\sigma$  of the mean magnitude.

§Number of observations.

||Observer's code: Neu (V. Neustroev team), Van (T. Vanmunster), Han (Hankasalmi Obs., by A. Oksanen), Trt (T. Tordai), KU1 (Kyoto U., campus obs.), deM (E. de Miguel), Aka (H. Akazawa, OUS) and AAVSO collaboration.

#Filter. "C" means no filter (clear).

**Table S2.** Times of superhump maxima in ASASSN-16eg.

| $E$ | max*       | error  | $O - C^\dagger$ | $N^\ddagger$ |
|-----|------------|--------|-----------------|--------------|
| 0   | 57494.1637 | 0.0010 | -0.0183         | 44           |
| 1   | 57494.2401 | 0.0005 | -0.0198         | 111          |
| 4   | 57494.4828 | 0.0003 | -0.0109         | 170          |
| 5   | 57494.5578 | 0.0002 | -0.0138         | 170          |
| 6   | 57494.6424 | 0.0006 | -0.0071         | 106          |
| 7   | 57494.7194 | 0.0004 | -0.0080         | 182          |
| 8   | 57494.7982 | 0.0003 | -0.0071         | 410          |
| 9   | 57494.8814 | 0.0003 | -0.0018         | 326          |
| 10  | 57494.9628 | 0.0002 | 0.0017          | 217          |
| 15  | 57495.3530 | 0.0002 | 0.0023          | 102          |
| 16  | 57495.4307 | 0.0001 | 0.0021          | 180          |
| 17  | 57495.5085 | 0.0001 | 0.0020          | 197          |
| 18  | 57495.5878 | 0.0002 | 0.0033          | 391          |
| 19  | 57495.6645 | 0.0002 | 0.0022          | 392          |
| 20  | 57495.7434 | 0.0001 | 0.0032          | 460          |
| 21  | 57495.8200 | 0.0001 | 0.0018          | 484          |
| 22  | 57495.8982 | 0.0001 | 0.0021          | 419          |
| 23  | 57495.9750 | 0.0002 | 0.0010          | 293          |
| 25  | 57496.1284 | 0.0005 | -0.0015         | 330          |
| 26  | 57496.2084 | 0.0005 | 0.0007          | 353          |
| 27  | 57496.2856 | 0.0002 | -0.0001         | 134          |
| 28  | 57496.3642 | 0.0001 | 0.0006          | 95           |
| 29  | 57496.4418 | 0.0001 | 0.0003          | 187          |
| 30  | 57496.5188 | 0.0001 | -0.0006         | 348          |
| 31  | 57496.5979 | 0.0001 | 0.0005          | 348          |
| 32  | 57496.6748 | 0.0001 | -0.0004         | 299          |
| 33  | 57496.7526 | 0.0001 | -0.0005         | 624          |
| 34  | 57496.8293 | 0.0001 | -0.0018         | 704          |
| 35  | 57496.9067 | 0.0001 | -0.0022         | 584          |
| 36  | 57496.9859 | 0.0002 | -0.0010         | 286          |
| 40  | 57497.2971 | 0.0002 | -0.0014         | 41           |
| 41  | 57497.3787 | 0.0006 | 0.0023          | 113          |
| 42  | 57497.4525 | 0.0004 | -0.0019         | 86           |
| 43  | 57497.5309 | 0.0003 | -0.0014         | 78           |
| 44  | 57497.6082 | 0.0003 | -0.0019         | 76           |
| 46  | 57497.7658 | 0.0002 | -0.0002         | 180          |
| 47  | 57497.8429 | 0.0002 | -0.0011         | 218          |
| 48  | 57497.9192 | 0.0002 | -0.0026         | 282          |
| 49  | 57497.9967 | 0.0002 | -0.0031         | 191          |
| 51  | 57498.1561 | 0.0002 | 0.0005          | 302          |
| 52  | 57498.2309 | 0.0001 | -0.0026         | 306          |
| 55  | 57498.4655 | 0.0002 | -0.0018         | 189          |
| 56  | 57498.5424 | 0.0001 | -0.0028         | 392          |
| 57  | 57498.6200 | 0.0002 | -0.0030         | 320          |
| 58  | 57498.6971 | 0.0002 | -0.0039         | 192          |
| 59  | 57498.7752 | 0.0002 | -0.0037         | 289          |
| 60  | 57498.8524 | 0.0002 | -0.0044         | 239          |

\*BJD-2400000.

 $^\dagger C = 2457496.4415 + 0.077913E$ . $^\ddagger$ Number of points used to determine the maximum.**Table S2.** Times of superhump maxima in ASASSN-16eg (continued).

| $E$ | max*       | error  | $O - C^\dagger$ | $N^\ddagger$ |
|-----|------------|--------|-----------------|--------------|
| 61  | 57498.9302 | 0.0002 | -0.0045         | 96           |
| 62  | 57499.0080 | 0.0003 | -0.0047         | 65           |
| 68  | 57499.4765 | 0.0003 | -0.0036         | 98           |
| 69  | 57499.5553 | 0.0002 | -0.0027         | 101          |
| 70  | 57499.6331 | 0.0003 | -0.0028         | 63           |
| 80  | 57500.4154 | 0.0004 | 0.0003          | 38           |
| 89  | 57501.1178 | 0.0004 | 0.0015          | 163          |
| 90  | 57501.1989 | 0.0005 | 0.0047          | 172          |
| 91  | 57501.2760 | 0.0002 | 0.0039          | 167          |
| 106 | 57502.4492 | 0.0005 | 0.0084          | 42           |
| 120 | 57503.5348 | 0.0004 | 0.0032          | 76           |
| 121 | 57503.6121 | 0.0004 | 0.0025          | 75           |
| 122 | 57503.6896 | 0.0005 | 0.0021          | 39           |
| 129 | 57504.2322 | 0.0002 | -0.0006         | 172          |
| 130 | 57504.3097 | 0.0004 | -0.0010         | 101          |
| 134 | 57504.6195 | 0.0004 | -0.0028         | 70           |
| 135 | 57504.7011 | 0.0008 | 0.0008          | 42           |
| 159 | 57506.5620 | 0.0004 | -0.0082         | 78           |
| 180 | 57508.1908 | 0.0013 | -0.0156         | 30           |
| 181 | 57508.2681 | 0.0006 | -0.0162         | 294          |

\*BJD-2400000.

 $^\dagger C = 2457496.4415 + 0.077913E$ . $^\ddagger$ Number of points used to determine the maximum.

**Table S3.** Times of superhump maxima in V1251 Cyg.

| $E$ | max*       | error  | $O - C^\dagger$ | $N^\ddagger$ |
|-----|------------|--------|-----------------|--------------|
| 0   | 54763.3947 | 0.0002 | -0.0055         | 48           |
| 1   | 54763.4681 | 0.0004 | -0.0080         | 80           |
| 3   | 54763.6234 | 0.0014 | -0.0047         | 39           |
| 4   | 54763.7010 | 0.0004 | -0.0030         | 93           |
| 5   | 54763.7784 | 0.0003 | -0.0016         | 89           |
| 12  | 54764.3114 | 0.0002 | -0.0003         | 273          |
| 13  | 54764.3862 | 0.0004 | -0.0014         | 296          |
| 14  | 54764.4629 | 0.0002 | -0.0007         | 326          |
| 16  | 54764.6151 | 0.0002 | -0.0005         | 28           |
| 17  | 54764.6918 | 0.0001 | 0.0003          | 220          |
| 18  | 54764.7670 | 0.0001 | -0.0005         | 201          |
| 26  | 54765.3739 | 0.0004 | -0.0012         | 108          |
| 27  | 54765.4514 | 0.0003 | 0.0003          | 131          |
| 28  | 54765.5271 | 0.0004 | -0.0000         | 141          |
| 29  | 54765.6038 | 0.0003 | 0.0008          | 183          |
| 30  | 54765.6786 | 0.0002 | -0.0004         | 174          |
| 31  | 54765.7539 | 0.0002 | -0.0010         | 118          |
| 32  | 54765.8296 | 0.0003 | -0.0013         | 40           |
| 38  | 54766.2831 | 0.0003 | -0.0036         | 80           |
| 39  | 54766.3603 | 0.0003 | -0.0024         | 143          |
| 40  | 54766.4363 | 0.0004 | -0.0023         | 86           |
| 42  | 54766.5860 | 0.0006 | -0.0045         | 20           |
| 43  | 54766.6621 | 0.0007 | -0.0044         | 28           |
| 44  | 54766.7391 | 0.0011 | -0.0033         | 29           |
| 45  | 54766.8149 | 0.0005 | -0.0035         | 26           |
| 47  | 54766.9679 | 0.0007 | -0.0025         | 127          |
| 49  | 54767.1186 | 0.0004 | -0.0036         | 178          |
| 54  | 54767.5010 | 0.0003 | -0.0011         | 99           |
| 56  | 54767.6526 | 0.0003 | -0.0014         | 104          |
| 57  | 54767.7286 | 0.0003 | -0.0014         | 106          |
| 60  | 54767.9571 | 0.0008 | -0.0007         | 419          |
| 63  | 54768.1858 | 0.0004 | 0.0001          | 74           |
| 64  | 54768.2610 | 0.0003 | -0.0006         | 122          |
| 65  | 54768.3374 | 0.0003 | -0.0002         | 126          |
| 66  | 54768.4136 | 0.0003 | 0.0001          | 126          |
| 67  | 54768.4878 | 0.0006 | -0.0018         | 79           |
| 69  | 54768.6412 | 0.0004 | -0.0003         | 79           |
| 70  | 54768.7177 | 0.0004 | 0.0003          | 79           |
| 73  | 54768.9473 | 0.0011 | 0.0020          | 87           |
| 76  | 54769.1724 | 0.0004 | -0.0008         | 46           |
| 77  | 54769.2510 | 0.0004 | 0.0018          | 86           |
| 78  | 54769.3265 | 0.0004 | 0.0014          | 87           |
| 79  | 54769.4022 | 0.0004 | 0.0011          | 80           |
| 80  | 54769.4758 | 0.0005 | -0.0012         | 83           |
| 86  | 54769.9294 | 0.0007 | -0.0034         | 268          |
| 87  | 54770.0064 | 0.0005 | -0.0024         | 373          |
| 90  | 54770.2353 | 0.0004 | -0.0014         | 81           |

\*BJD-2400000.

 $^\dagger C = 2454765.6790 + 0.0759607E$ . $^\ddagger$ Number of points used to determine the maximum.**Table S3.** Times of superhump maxima in V1251 Cyg (continued).

| $E$ | max*       | error  | $O - C^\dagger$ | $N^\ddagger$ |
|-----|------------|--------|-----------------|--------------|
| 91  | 54770.3104 | 0.0004 | -0.0022         | 76           |
| 92  | 54770.3875 | 0.0004 | -0.0011         | 59           |
| 93  | 54770.4626 | 0.0005 | -0.0019         | 58           |
| 113 | 54771.9752 | 0.0013 | -0.0085         | 278          |
| 114 | 54772.0501 | 0.0003 | -0.0096         | 157          |
| 117 | 54772.2791 | 0.0005 | -0.0085         | 76           |
| 122 | 54772.6556 | 0.0005 | -0.0118         | 79           |
| 123 | 54772.7308 | 0.0005 | -0.0125         | 71           |
| 144 | 54774.3232 | 0.0006 | -0.0154         | 136          |
| 145 | 54774.3968 | 0.0004 | -0.0177         | 135          |
| 146 | 54774.4716 | 0.0006 | -0.0189         | 46           |

\*BJD-2400000.

 $^\dagger C = 2454765.6790 + 0.0759607E$ . $^\ddagger$ Number of points used to determine the maximum.

**Table S4.** Times of superhump maxima in RZ Leo.

| $E$ | max*       | error  | $O - C^\dagger$ | $N^\ddagger$ |
|-----|------------|--------|-----------------|--------------|
| 0   | 51901.1568 | 0.0009 | -0.0201         | 110          |
| 1   | 51901.2307 | 0.0014 | -0.0246         | 145          |
| 2   | 51901.3041 | 0.0007 | -0.0298         | 148          |
| 5   | 51901.5444 | 0.0008 | -0.0252         | 171          |
| 6   | 51901.6245 | 0.0006 | -0.0236         | 185          |
| 13  | 51902.1980 | 0.0003 | 0.0003          | 208          |
| 14  | 51902.2755 | 0.0003 | -0.0008         | 203          |
| 15  | 51902.3542 | 0.0003 | -0.0006         | 171          |
| 18  | 51902.5902 | 0.0006 | -0.0003         | 134          |
| 23  | 51902.9853 | 0.0005 | 0.0022          | 41           |
| 24  | 51903.0665 | 0.0003 | 0.0049          | 41           |
| 25  | 51903.1455 | 0.0006 | 0.0053          | 117          |
| 26  | 51903.2191 | 0.0003 | 0.0005          | 169          |
| 27  | 51903.2972 | 0.0004 | -0.0000         | 205          |
| 28  | 51903.3772 | 0.0006 | 0.0014          | 108          |
| 39  | 51904.2464 | 0.0005 | 0.0068          | 83           |
| 40  | 51904.3248 | 0.0003 | 0.0066          | 114          |
| 51  | 51905.1840 | 0.0003 | 0.0019          | 183          |
| 52  | 51905.2611 | 0.0003 | 0.0006          | 176          |
| 53  | 51905.3400 | 0.0004 | 0.0009          | 146          |
| 64  | 51906.2083 | 0.0005 | 0.0054          | 150          |
| 65  | 51906.2856 | 0.0003 | 0.0041          | 215          |
| 66  | 51906.3637 | 0.0009 | 0.0037          | 122          |
| 76  | 51907.1514 | 0.0004 | 0.0061          | 146          |
| 77  | 51907.2294 | 0.0007 | 0.0055          | 108          |
| 84  | 51907.7799 | 0.0005 | 0.0064          | 35           |
| 85  | 51907.8599 | 0.0008 | 0.0078          | 17           |
| 86  | 51907.9387 | 0.0006 | 0.0080          | 17           |
| 89  | 51908.1751 | 0.0005 | 0.0089          | 149          |
| 90  | 51908.2559 | 0.0004 | 0.0111          | 285          |
| 91  | 51908.3329 | 0.0003 | 0.0096          | 257          |
| 99  | 51908.9644 | 0.0004 | 0.0128          | 40           |
| 100 | 51909.0404 | 0.0004 | 0.0103          | 40           |
| 111 | 51909.9016 | 0.0006 | 0.0076          | 33           |
| 112 | 51909.9750 | 0.0007 | 0.0025          | 40           |
| 113 | 51910.0559 | 0.0003 | 0.0049          | 42           |
| 128 | 51911.2277 | 0.0011 | -0.0013         | 221          |
| 129 | 51911.3055 | 0.0014 | -0.0021         | 219          |
| 153 | 51913.1815 | 0.0009 | -0.0108         | 200          |
| 154 | 51913.2620 | 0.0007 | -0.0089         | 219          |
| 155 | 51913.3423 | 0.0007 | -0.0070         | 225          |
| 167 | 51914.2836 | 0.0022 | -0.0082         | 64           |
| 168 | 51914.3615 | 0.0021 | -0.0088         | 88           |

\*BJD-2400000.

 $^\dagger C = 2451901.175544 + 0.078533E$ . $^\ddagger$ Number of points used to determine the maximum.**Table S5.** Times of superhump maxima in BC UMa.

| $E$ | max*       | error  | $O - C^\dagger$ | $N^\ddagger$ |
|-----|------------|--------|-----------------|--------------|
| 0   | 52674.1092 | 0.0005 | 0.0011          | 55           |
| 1   | 52674.1745 | 0.0002 | 0.0018          | 70           |
| 2   | 52674.2384 | 0.0002 | 0.0012          | 118          |
| 3   | 52674.3020 | 0.0003 | 0.0003          | 74           |
| 4   | 52674.3679 | 0.0002 | 0.0015          | 156          |
| 5   | 52674.4330 | 0.0003 | 0.0021          | 66           |
| 6   | 52674.4979 | 0.0002 | 0.0024          | 67           |
| 31  | 52676.1071 | 0.0005 | -0.0027         | 57           |
| 32  | 52676.1718 | 0.0006 | -0.0025         | 68           |
| 33  | 52676.2372 | 0.0006 | -0.0017         | 150          |
| 34  | 52676.2992 | 0.0007 | -0.0043         | 51           |
| 35  | 52676.3646 | 0.0003 | -0.0035         | 117          |
| 36  | 52676.4291 | 0.0004 | -0.0036         | 67           |
| 37  | 52676.4945 | 0.0005 | -0.0027         | 61           |
| 47  | 52677.1405 | 0.0005 | -0.0025         | 173          |
| 48  | 52677.2052 | 0.0005 | -0.0024         | 181          |
| 49  | 52677.2683 | 0.0004 | -0.0038         | 199          |
| 50  | 52677.3353 | 0.0006 | -0.0014         | 135          |
| 52  | 52677.4652 | 0.0013 | -0.0006         | 42           |
| 63  | 52678.1748 | 0.0008 | -0.0014         | 107          |
| 65  | 52678.3023 | 0.0013 | -0.0030         | 92           |
| 93  | 52680.1127 | 0.0006 | -0.0006         | 178          |
| 95  | 52680.2403 | 0.0010 | -0.0021         | 148          |
| 96  | 52680.3078 | 0.0014 | 0.0008          | 66           |
| 97  | 52680.3712 | 0.0008 | -0.0004         | 81           |
| 98  | 52680.4368 | 0.0006 | 0.0006          | 133          |
| 99  | 52680.5002 | 0.0011 | -0.0005         | 80           |
| 108 | 52681.0751 | 0.0017 | -0.0069         | 80           |
| 109 | 52681.1407 | 0.0010 | -0.0058         | 76           |
| 110 | 52681.2066 | 0.0002 | -0.0045         | 316          |
| 113 | 52681.3981 | 0.0007 | -0.0067         | 67           |
| 124 | 52682.1098 | 0.0020 | -0.0053         | 102          |
| 127 | 52682.2962 | 0.0014 | -0.0126         | 63           |
| 128 | 52682.3596 | 0.0014 | -0.0138         | 85           |
| 139 | 52683.0692 | 0.0015 | -0.0145         | 115          |
| 140 | 52683.1330 | 0.0022 | -0.0153         | 159          |
| 141 | 52683.1961 | 0.0011 | -0.0167         | 333          |
| 142 | 52683.2625 | 0.0005 | -0.0149         | 262          |
| 143 | 52683.3230 | 0.0009 | -0.0189         | 142          |
| 144 | 52683.3923 | 0.0016 | -0.0143         | 87           |
| 145 | 52683.4547 | 0.0010 | -0.0164         | 54           |
| 160 | 52684.4141 | 0.0014 | -0.0256         | 44           |
| 161 | 52684.4808 | 0.0026 | -0.0235         | 44           |

\*BJD-2400000.

 $^\dagger C = 2452674.2372 + 0.0645728E$ . $^\ddagger$ Number of points used to determine the maximum.

**Table S6.** Times of superhump maxima in MASTER J004527.

| $E$ | max*       | error  | $O - C^\dagger$ | $N^\ddagger$ |
|-----|------------|--------|-----------------|--------------|
| 0   | 56554.3615 | 0.0004 | -0.0151         | 95           |
| 4   | 56554.6863 | 0.0002 | -0.0111         | 234          |
| 5   | 56554.7697 | 0.0003 | -0.0079         | 147          |
| 6   | 56554.8514 | 0.0003 | -0.0064         | 129          |
| 7   | 56554.9367 | 0.0008 | -0.0013         | 74           |
| 12  | 56555.3362 | 0.0001 | -0.0027         | 204          |
| 13  | 56555.4176 | 0.0001 | -0.0015         | 287          |
| 14  | 56555.4968 | 0.0001 | -0.0026         | 381          |
| 15  | 56555.5763 | 0.0001 | -0.0033         | 312          |
| 16  | 56555.6567 | 0.0002 | -0.0030         | 319          |
| 19  | 56555.8984 | 0.0003 | -0.0019         | 62           |
| 20  | 56555.9783 | 0.0002 | -0.0022         | 64           |
| 25  | 56556.3799 | 0.0001 | -0.0016         | 280          |
| 26  | 56556.4608 | 0.0001 | -0.0009         | 279          |
| 27  | 56556.5419 | 0.0002 | 0.0000          | 172          |
| 28  | 56556.6222 | 0.0001 | 0.0001          | 200          |
| 29  | 56556.7031 | 0.0002 | 0.0009          | 187          |
| 30  | 56556.7821 | 0.0003 | -0.0004         | 188          |
| 31  | 56556.8632 | 0.0002 | 0.0005          | 203          |
| 32  | 56556.9438 | 0.0003 | 0.0009          | 63           |
| 36  | 56557.2658 | 0.0002 | 0.0021          | 312          |
| 40  | 56557.5857 | 0.0004 | 0.0012          | 62           |
| 41  | 56557.6658 | 0.0003 | 0.0011          | 69           |
| 42  | 56557.7471 | 0.0003 | 0.0023          | 61           |
| 43  | 56557.8253 | 0.0003 | 0.0003          | 71           |
| 44  | 56557.9070 | 0.0004 | 0.0018          | 71           |
| 47  | 56558.1487 | 0.0002 | 0.0029          | 120          |
| 48  | 56558.2291 | 0.0002 | 0.0031          | 212          |
| 49  | 56558.3103 | 0.0002 | 0.0041          | 237          |
| 50  | 56558.3881 | 0.0001 | 0.0018          | 187          |
| 51  | 56558.4681 | 0.0001 | 0.0015          | 196          |
| 52  | 56558.5481 | 0.0002 | 0.0013          | 223          |
| 53  | 56558.6279 | 0.0002 | 0.0009          | 255          |
| 54  | 56558.7087 | 0.0002 | 0.0015          | 139          |
| 55  | 56558.7886 | 0.0003 | 0.0013          | 62           |
| 60  | 56559.1900 | 0.0001 | 0.0016          | 210          |
| 61  | 56559.2689 | 0.0002 | 0.0004          | 263          |
| 62  | 56559.3492 | 0.0002 | 0.0005          | 163          |
| 63  | 56559.4307 | 0.0002 | 0.0018          | 128          |
| 64  | 56559.5097 | 0.0002 | 0.0005          | 170          |
| 65  | 56559.5889 | 0.0004 | -0.0004         | 67           |
| 66  | 56559.6693 | 0.0002 | -0.0002         | 206          |
| 67  | 56559.7488 | 0.0002 | -0.0009         | 189          |
| 68  | 56559.8289 | 0.0003 | -0.0010         | 74           |
| 69  | 56559.9088 | 0.0005 | -0.0013         | 71           |
| 72  | 56560.1490 | 0.0002 | -0.0017         | 110          |
| 73  | 56560.2292 | 0.0002 | -0.0016         | 137          |

\*BJD-2400000.

 $^\dagger C = 2456556.3815 + 0.0801953E$ . $^\ddagger$ Number of points used to determine the maximum.**Table S6.** Times of superhump maxima in MASTER J004527 (continued).

| $E$ | max*       | error  | $O - C^\dagger$ | $N^\ddagger$ |
|-----|------------|--------|-----------------|--------------|
| 77  | 56560.5501 | 0.0005 | -0.0016         | 57           |
| 80  | 56560.7899 | 0.0005 | -0.0023         | 61           |
| 81  | 56560.8685 | 0.0005 | -0.0039         | 69           |
| 87  | 56561.3516 | 0.0007 | -0.0020         | 104          |
| 88  | 56561.4289 | 0.0002 | -0.0049         | 108          |
| 90  | 56561.5884 | 0.0007 | -0.0058         | 69           |
| 91  | 56561.6684 | 0.0004 | -0.0060         | 69           |
| 92  | 56561.7487 | 0.0007 | -0.0059         | 53           |
| 93  | 56561.8290 | 0.0005 | -0.0058         | 72           |
| 94  | 56561.9088 | 0.0006 | -0.0061         | 71           |
| 98  | 56562.2279 | 0.0003 | -0.0078         | 154          |
| 99  | 56562.3124 | 0.0004 | -0.0035         | 126          |
| 102 | 56562.5482 | 0.0007 | -0.0083         | 57           |
| 103 | 56562.6290 | 0.0006 | -0.0077         | 64           |
| 104 | 56562.7083 | 0.0008 | -0.0086         | 52           |
| 105 | 56562.7885 | 0.0007 | -0.0086         | 64           |
| 106 | 56562.8679 | 0.0005 | -0.0094         | 70           |
| 110 | 56563.1897 | 0.0004 | -0.0084         | 74           |
| 111 | 56563.2715 | 0.0006 | -0.0068         | 84           |
| 112 | 56563.3480 | 0.0005 | -0.0105         | 139          |
| 113 | 56563.4279 | 0.0004 | -0.0108         | 104          |
| 115 | 56563.5883 | 0.0010 | -0.0108         | 63           |
| 116 | 56563.6714 | 0.0008 | -0.0079         | 121          |
| 117 | 56563.7501 | 0.0007 | -0.0094         | 88           |
| 118 | 56563.8278 | 0.0010 | -0.0118         | 72           |
| 119 | 56563.9077 | 0.0012 | -0.0122         | 71           |
| 122 | 56564.1450 | 0.0003 | -0.0154         | 65           |
| 123 | 56564.2246 | 0.0009 | -0.0160         | 84           |

\*BJD-2400000.

 $^\dagger C = 2456556.3815 + 0.0801953E$ . $^\ddagger$ Number of points used to determine the maximum.
